# Supplementary material for: Hidden Symmetries in Gravity : Black holes and other minisuperspaces
Source: arXiv:2211.04909 source file (2022-11-09)
Supplement: Supplementary file 1 [file app_3.tex]

\chapter{Lapse function, time diffeomorphisms and charges}
\label{app:3_time_diffeos}

Let us consider the simple example of the Lagrangian
\be
L=\f{1}{2N}\dot{q}^2+\dot{N}\Pi-\mu\Pi.
\ee
Here we have added from the onset a momentum $\Pi$ for $N$, together with a multiplier $\mu$ enforcing the constraint $\Pi\approx0$. The potential will play no role in this discussion and we have therefore removed it. The variation is
\be
\delta L=\f{1}{N^2}\big(\dot{q}\dot{N}-N\ddot{q}\big)\delta q-\left(\f{\dot{q}^2}{2N^2}+\dot{\Pi}\right)\delta N+(\dot{N}-\mu)\delta\Pi-\delta\mu\Pi+\dot{\theta},
\ee
where
\be
\theta=\f{\dot{q}}{N}\delta q+\Pi\delta N.
\ee
This Lagrangian is invariant under the symmetry
\be\label{alpha symmetry}
\delta_\alpha q=\alpha\dot{q},
\q\q
\delta_\alpha N=\alpha\dot{N}+\dot{\alpha}N=\partial_t(\alpha N),
\q\q
\delta_\alpha\Pi=0,
\q\q
\delta_\alpha\mu=\delta_\alpha\dot{N}.
\ee
The Hamiltonian is
\be
H=\f{1}{2}Np^2+\mu\Pi,
\q\q
p=\f{\dot{q}}{N}.
\ee
We can compute the generator of \eqref{alpha symmetry} with the covariant phase space formalism and $\Omega=\delta\theta$. Using the fact that $\delta_\alpha(\dot{q}/N)\approx0$ thanks to the equation of motion imposed by $q$, we find
\be
-\delta_\alpha\ipp\Omega\approx\alpha\dot{q}\delta\left(\f{\dot{q}}{N}\right)+\partial_t(\alpha N)\delta\Pi.
\ee
One can see that this is not integrable, and that integrability can be achieved with the field-dependent redefinition $\alpha=\eps/N$, for which we find a generator given by
\be
G(\eps)=\f{1}{2}\eps p^2+\dot{\eps}\Pi.
\ee
The Poisson bracket of this generator with $q$ and $N$ does indeed generate \eqref{alpha symmetry} with $\alpha=\eps/N$. Note however that there is a priori no obstruction to acting with $G(\alpha N)=\alpha H+\dot{\alpha}N\Pi$, which generates the initial (non-integrable) transformation \eqref{alpha symmetry}.

We have
\be
V=\f{q\Pi}{p}-\f{N^3p^2}{2\mu^2}+\f{3Nqp}{2\mu},\q C=\lb V,H\rb=qp+N\Pi,\q\lb C,V\rb=-V,\q\lb C,H\rb=H,
\ee
which implies that $Q=C-tH$ is conserved. It generates the symmetry
\be
\delta_\alpha q=q-t\dot{q},
\q\q
\delta_\alpha N=N-t\dot{N},
\q\q
\delta_\alpha\Pi=0,
\q\q
\delta_\alpha\mu=\delta_\alpha\dot{N},
\ee
which however is known only for $\alpha=1$. What is the extension to $\alpha(t)$?

$$**********************************************************$$

$$\f{\de G(\eps)}{\de t}=\f{\partial G(\eps)}{\partial t}+\lb G(\eps),H\rb=\f{1}{2}\dot{\eps}p^2+\ddot{\eps}\Pi-\f{1}{2}\dot{\eps}p^2=\ddot{\eps}\Pi\approx0.$$

$$V=q^2+\f{2\eps}{\dot{\eps}}N^2\Pi,\q C=\lb V,G(\eps)\rb=2\eps(qp+2N\Pi)\q\lb C,V\rb=-4\eps V,\q\lb C,G(\eps)\rb=4\eps G(\eps)$$
